# Supplementary material for: On the Vulnerability of Fairness Constrained Learning to Malicious Noise
Source: arXiv:2307.11892 source file (2024-08-22)
Supplement: Supplementary file 1 [file supplement.tex]

\documentclass[twoside]{article}

\usepackage{aistats2024}
% If your paper is accepted, change the options for the package
% aistats2022 as follows:
%
%\usepackage[accepted]{aistats2024}
%
% This option will print headings for the title of your paper and
% headings for the authors names, plus a copyright note at the end of
% the first column of the first page.

% If you set papersize explicitly, activate the following three lines:
%\special{papersize = 8.5in, 11in}
%\setlength{\pdfpageheight}{11in}
%\setlength{\pdfpagewidth}{8.5in}

% If you use natbib package, activate the following three lines:
%\usepackage[round]{natbib}
%\renewcommand{\bibname}{References}
%\renewcommand{\bibsection}{\subsubsection*{\bibname}}

% If you use BibTeX in apalike style, activate the following line:
%\bibliographystyle{apalike}

\include{notations}
\usepackage{mkolar_definitions}
\usepackage{multirow}
\usepackage{amsmath}

\usepackage{color-edits}[suppress]
\addauthor[suppress]{pco}{purple}
\addauthor[suppress]{kms}{orange}
\addauthor[suppress]{as}{cyan}
\usepackage{alg}
\usepackage{multirow}
\usepackage{graphicx}

\usepackage[utf8]{inputenc} % allow utf-8 input
\usepackage{amsmath}
\usepackage{amsfonts}
\usepackage{amssymb}
\usepackage{bbm}

\usepackage[T1]{fontenc}    % use 8-bit T1 fonts
\usepackage{hyperref}       % hyperlinks
\usepackage{url}            % simple URL typesetting
\usepackage{booktabs}       % professional-quality tables
\usepackage{amsfonts}       % blackboard math symbols
\usepackage{nicefrac}       % compact symbols for 1/2, etc.
\usepackage{microtype}      % microtypography
\usepackage{xcolor}         % colors
\usepackage{float}

\begin{document}

% If your paper is accepted and the title of your paper is very long,
% the style will print as headings an error message. Use the following
% command to supply a shorter title of your paper so that it can be
% used as headings.
%
%\runningtitle{I use this title instead because the last one was very long}

% If your paper is accepted and the number of authors is large, the
% style will print as headings an error message. Use the following
% command to supply a shorter version of the authors names so that
% they can be used as headings (for example, use only the surnames)
%
%\runningauthor{Surname 1, Surname 2, Surname 3, ...., Surname n}

% Supplementary material: To improve readability, you must use a single-column format for the supplementary material.
\onecolumn
\aistatstitle{Instructions for Paper Submissions to AISTATS 2024: \\
Supplementary Materials}

% \section{Fairness Notions}
% \label{fairtable}
% \begin{center}
% \begin{tabular}{ |p{4cm}||p{9cm}| }
%  \hline
%  \multicolumn{2}{|c|}{ Fairness Constraints}\\
%  \hline
%  Demographic Parity \cite{dwork2012fairness} & $ P_{(x,y) \sim \DA} [h(x)=1]= P_{(x,y) \sim \DB} [h(x)=1] $  \\
%  \hline 
%  Equal Opportunity \cite{hardt16} & $ P_{(x,y) \sim \DA} [h(x)=1| y=1 ]= P_{(x,y) \sim \DB} [h(x)=1| y=1 ] $ \\
%  \hline
%  Equalized Odds \cite{hardt16} &   $P_{(x,y) \sim \DA} [h(x)=1| y=1 ]= P_{(x,y) \sim \DB} [h(x)=1| y=1 ]$ and \\
%   & $P_{(x,y) \sim \DA} [h(x)=1| y=0 ]= P_{(x,y) \sim \DB} [h(x)=1| y=0 ]$ \\
%   \hline
%   Predictive Parity \cite{chouldechova2017fair} & $P_{(x,y) \sim \DA} [y=1| h(x)=1 ]= P_{(x,y) \sim \DB} [y=1| h(x)=1 ]$ \\
% \hline
% Calibration\footnote{$h:\mathcal{X} \rightarrow [0,1]$} \cite{klein16,dawid} & $ \forall r \in [0,1],\quad  r = \mathbb{E}_{x,y \sim \mathcal{D}} [y|h(x)=r] $\\
% \hline
% \end{tabular}
% \end{center}

\section{Proofs}

\input{sections/parity}

\input{sections/eopp}

\input{sections/eodds}

\section{Calibration Proofs}

\input{sections/calibproof}

\input{sections/minimax}

\input{sections/multgroup}
\vfill

\end{document}
